# Supplementary material for: Accelerating Plasmonic Hydrogen Sensors for Inert Gas Environments by Transformer-Based Deep Learning
Source: arXiv:2312.15372 ancillary file (2023-12-23)
Supplement: Supplementary file 1 [file supporting-information.pdf]

# Supporting Information

## Accelerating Plasmonic Hydrogen Sensors in Inert Gas Environments by Transformer-Based Deep Learning

Viktor Martvall[1], Henrik Klein Moberg[1], Athanasios Theodoridis[1], David Tomeček[1], Pernilla Ekborg-Tanner[1], Sara Nilsson[1], Giovanni Volpe[2], Paul Erhart[1,*], and Christoph Langhammer[1,†]

[1] *Department of Physics, Chalmers University of Technology, SE-412 96 Gothenburg, Sweden*
[2] *Department of Physics, University of Gothenburg, 412 96 Gothenburg, Sweden*
[*] *erhart@chalmers.se*
[†] *clangham@chalmers.se*

# Contents

**Supplementary Notes** **2**
S1. Hydrogenation protocols . . . 2
S2. Data pre-processing . . . 2
S3. SotA analysis . . . 2

**Supplementary Figures** **3**
S1. Experimental setup . . . 3
S2. Gas background quadrupole mass spectrometer measurements . . . 4
S3. Gas background quadrupole mass spectrometer measurements . . . 5
S4. Step wise hydrogenation measurements . . . 6
S5. Linear and exponential hydrogenation measurements . . . 6
S6. Calibration function for step-wise increases/decreases . . . 7
S7. Calibration function applied to the test data . . . 7
S8. Calibration function for linear/exponential increases/decreases . . . 8
S9. Calibration function applied to the test data . . . 8
S10. Time series length for models optimized for accelerating sensor response . . . 8
S11. Time series length for models optimized for leak detection . . . 9
S12. Different pre-processing methods . . . 9
S13. Impact of using different pre-processing methods . . . 10
S14. Schematic illustration of the deep learning architecture used in this work . . . 10
S15. Comparison of LEMAS and SotA analysis for step-wise increases in test data . . . 11
S16. Initial prediction of mean and standard deviation by LEMAS for step-wise increases in test data . . . 12
S17. Comparison of LEMAS and SotA analysis for exponential leak rates in test data . . . 13

**Supplementary Tables** **14**
S1. Hyperparameters used for all models . . . 14

**Supplementary References** **14**

# Supplementary Notes

## Supplementary Note S1: Hydrogenation protocols

The hydrogenation protocols were as follows: 5 pulses of 1.97 vol.% $H_2$ concentration were introduced at the beginning of each measurement, in order to activate the nanodisks. For the step wise hydrogen profile (Fig. S4), 3 different measurements were performed which consisted of a logarithmic distribution of $H_2$ pulses (14 steps increase/decrease, 0.06 vol.% $H_2$ minimum and 1.97 vol.% $H_2$ maximum concentration), where the pulse durations were set to 5 min, 10 min and 15 min. The time between pulses was 30 min for all measurements.

For the linear hydrogen profile (Fig. S5a), the $H_2$ concentration was slowly increased linearly to a maximal concentration. For each of the ramp up/down cycles, the maximum concentrations were: 0.09, 0.13, 0.19, 0.28, 0.41, 0.61, 0.90, 1.33, 1.97 vol.% $H_2$.The ramp-up/down duration was 1 hour. The maximal concentrations were increasing after each ramping up/down and therefore the hydrogen increase rate was changing as well. For the exponential hydrogen profile (Fig. S5b) the $H_2$ concentration was increased exponentially to a maximal concentration instead of linearly. The duration of the ramp-up/down was 1 hour and the same maximum concentrations were used.

## Supplementary Note S2: Data pre-processing

Due to variations in the spectra from different measurements (see Fig. S12), it was necessary to pre-process the data before training a model (see Data pre-processing of the main paper). Initially, we only considered one pre-processing method (wavelength dependent min-max normalization), however, as seen by the blue curve in Fig. S13 this caused errors in the model predictions, which are likely due to the pre-processed spectra for similar $H_2$ concentration being relatively similar. Sequentially, we therefore added standard normal variate standardization (orange curve in Fig. S13), global min-max normalization (green curve in Fig. S13) and level scaling (red curve in Fig. S13). By using all four pre-processing methods the model accuracy increases substantially.

## Supplementary Note S3: SotA analysis

To obtain the calibration curve for the step-wise increases we used the measurement illustrated in Fig. S4a. For each pulse, we extracted the steady-state centroid shift as well as the $H_2$ concentration (Fig. S6). The motivation behind only using the steady-state centroid shift is that a unique mapping between the centroid shift and the $H_2$ concentration does not exist during the transient state. Then we minimized the mean absolute relative error and obtained $a = 0.334$ and $b = 2.91$ (see Eq. (1)). In Fig. S6 we illustrate the use of the obtained calibration function for predicting the $H_2$ concentration on the measurement used for testing LSTR Ensemble Model for Accelerated Sensing (LEMAS) (Fig. S4a). The mean absolute relative error of the state-of-the-art (SotA) analysis for this measurement is $14.73 \times 10^{-3}$ vol.% $H_2$, which is higher than the mean absolute relative error of LEMAS being $1.048 \times 10^{-3}$ vol.% $H_2$, showing that LEMAS has a higher accuracy.

To obtain the calibration curve for the linear/exponential increases we used the measurement consisting of linear increases/decreases (Fig. S5a). Here, we used the entire measurement to obtain a calibration curve, as the $H_2$ concentration changes slower than the response time of the system (Fig. S8). Then we minimized the mean absolute relative error and obtained $a = 0.40$ and $b = 2.51$. In Fig. S9 we illustrate the use of the obtained calibration function for predicting the $H_2$ concentration on the measurement used for testing LEMAS (Fig. S5b). The mean absolute relative error of the SotA analysis for this measurement is $13.43 \times 10^{-3}$ vol.% $H_2$, which is higher than the mean absolute relative error of LEMAS being $7.4 \times 10^{-3}$ vol.% $H_2$, confirming again that LEMAS has a higher accuracy.

## Supplementary Figures

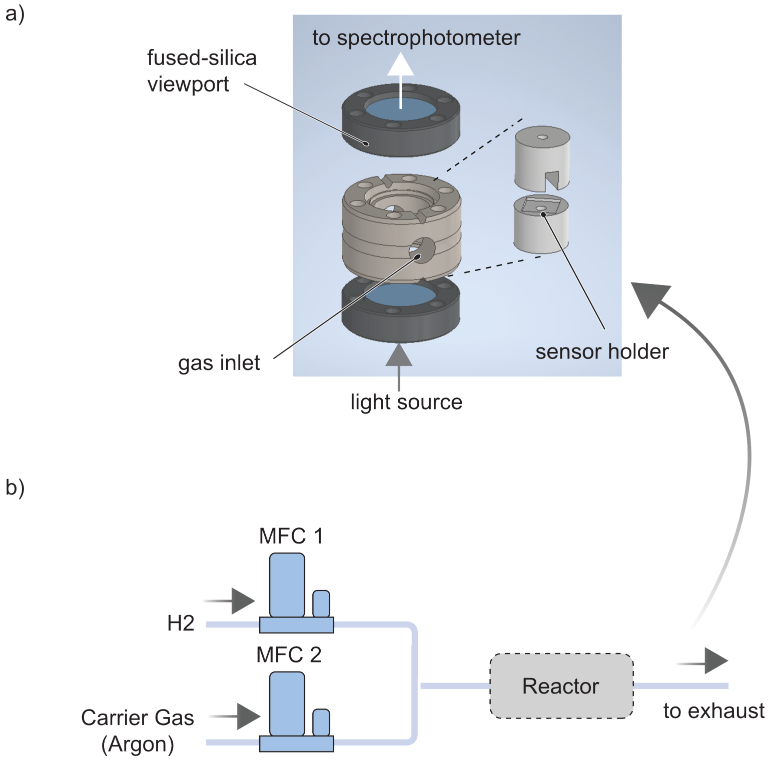


Figure S1: **Experimental setup.** Schematic illustration of the (a) reaction chamber and (b) gas mixing system. Adapted with permission from Ref. 1.

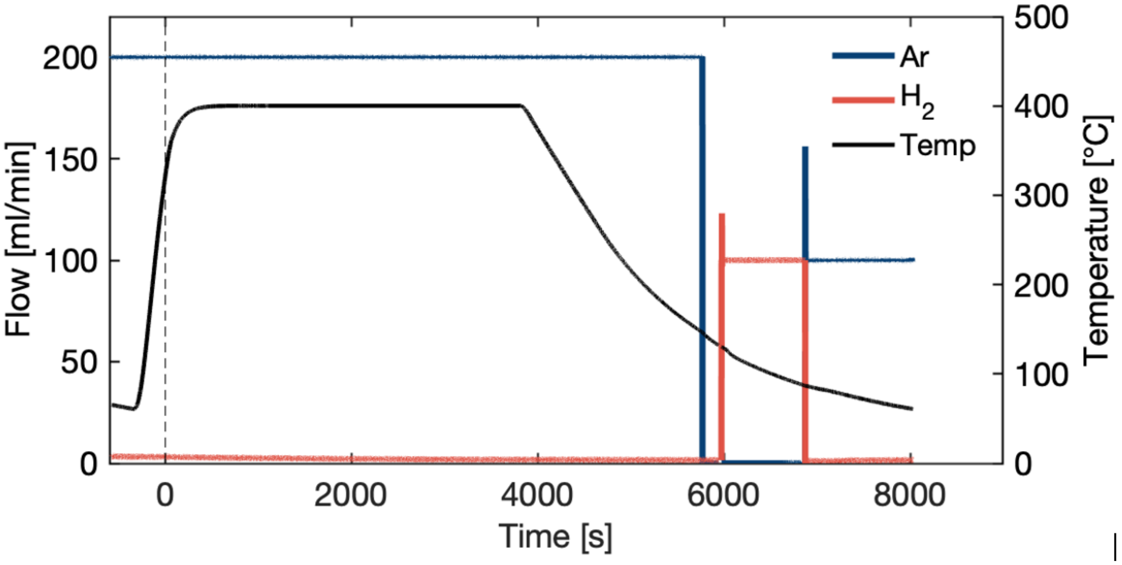


Figure S2: **Gas background quadrupole mass spectrometer measurements.** The gas flows of 100 % Ar (blue, left y-axis) followed by 100 % $H_2$ (red, left y-axis) and temperature (black, right y-axis) during the quadrupole mass spectrometer (QMS) measurements of the concentrations of possible trace gases in the mixture. The temperature was first increased to 400 °C in 100 % Ar flow, to desorb possible absorbed gases in the flow reactor. This was followed by one 15 minutes 100 % $H_2$ pulse, and again one pulse of 100 % Ar. The QMS measurement was started at time 0, marked by the dashed line.

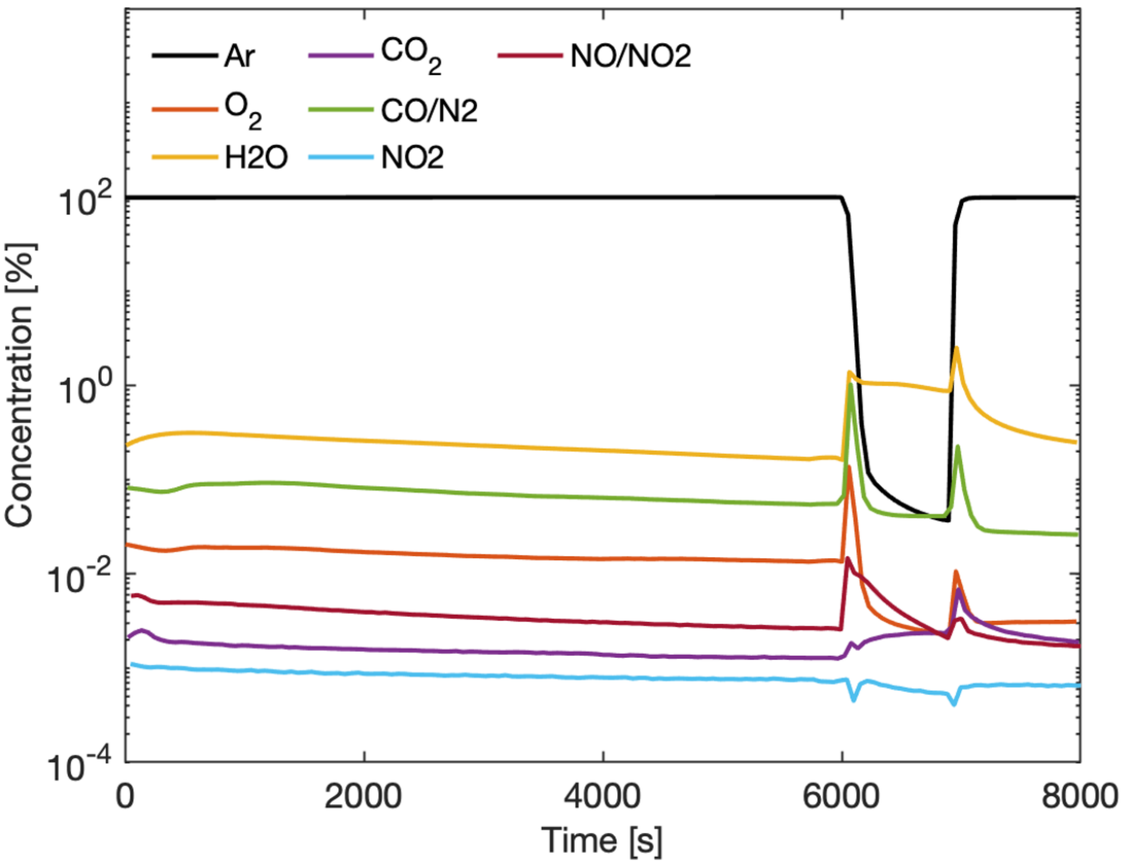


Figure S3: **Gas background quadrupole mass spectrometer measurements.** The concentrations of Ar and the trace gases during the Ar and H2 pulses in Fig. S2. The concentrations of the trace gases at the end of the Ar pulse at 8000 s were 99.7 % Ar, 0.26 % $H_2O$, 0.027 % CO or $N_2$, 31 ppm $O_2$, 18 ppm NO, and 6.6 ppm $NO_2$.

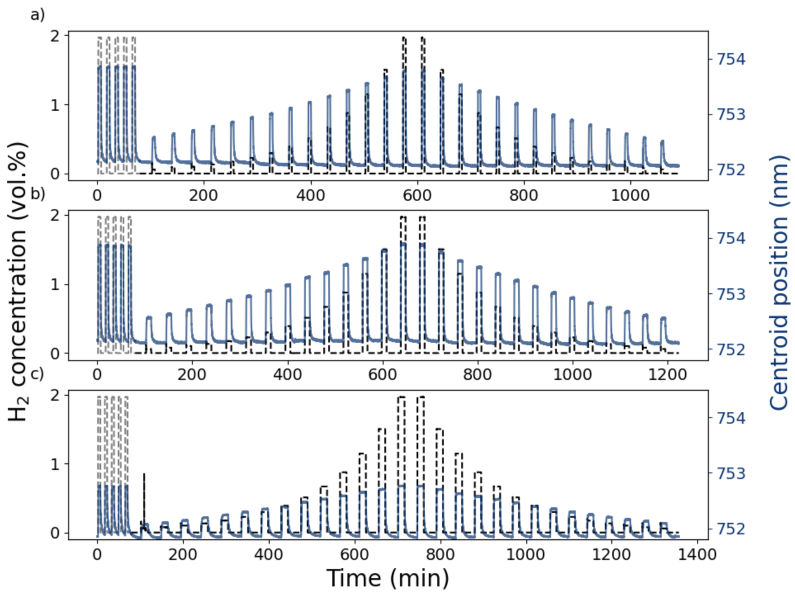


Figure S4: **Step wise hydrogenation measurements.** Hydrogenation protocol for the step wise increase/decrease, alongside the measured centroid shift. (a) 5 min, (b) 10 min, (c) 15 min of pulse duration followed by 30 minutes between each pulse for all measurements.

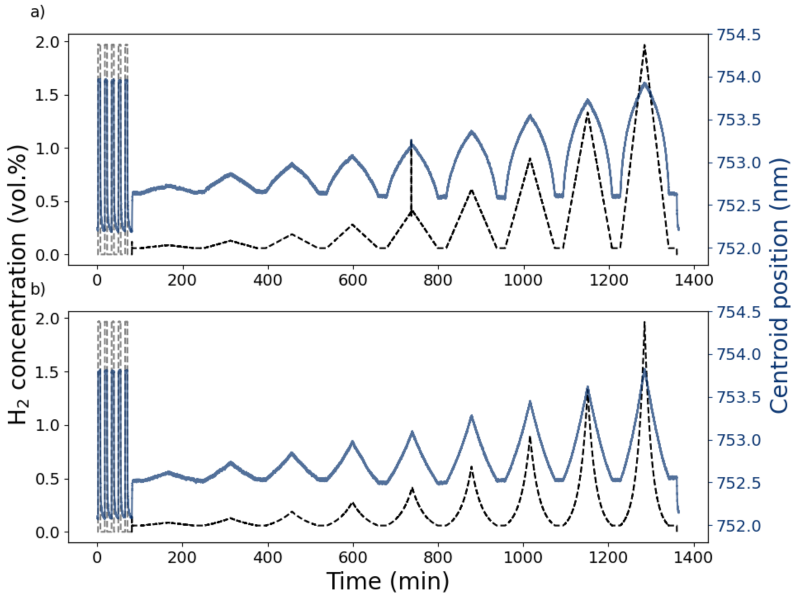


Figure S5: **Linear and exponential hydrogenation measurements.** Hydrogenation protocol for the (a) linear and (b) exponential increase/decrease alongside the measured centroid shift. The ramp-up/down duration for each cycle was 1 h.

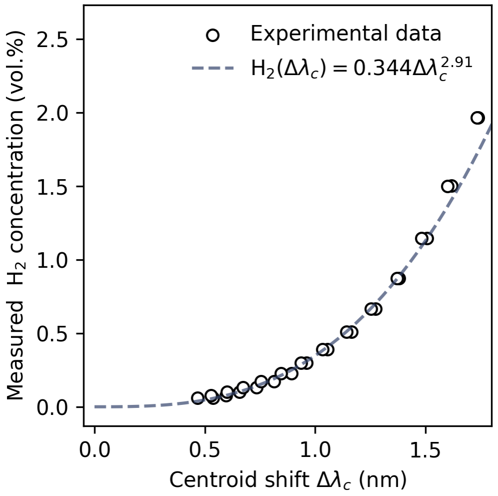


Figure S6: **Calibration function for step-wise increases/decreases.** Experimental data used from measurement Fig. S4a to fit the calibration function for the step-wise increases and the obtained calibration function.

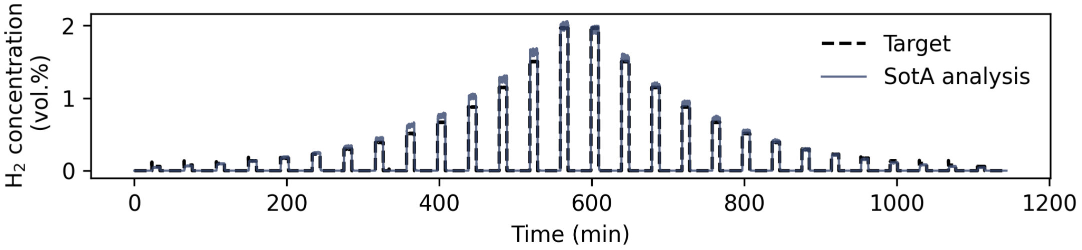


Figure S7: **Calibration function applied to the test data.** Calibration function obtained from Fig. S6 used on the test data, measurement Fig. S4b.

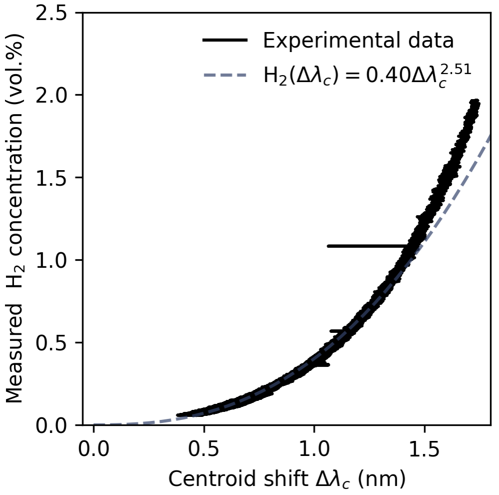


Figure S8: **Calibration function for linear/exponential increases/decreases .** Experimental data used from measurement Fig. S5a to fit the calibration function for the linear/exponential increases and the obtained calibration function.

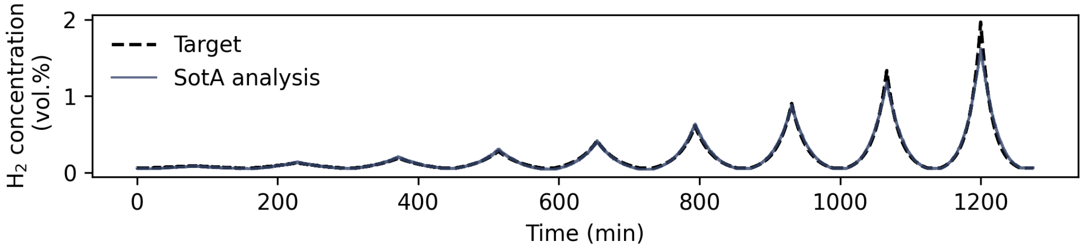


Figure S9: **Calibration function applied to the test data.** Calibration function obtained from Fig. S8 used on the test data, measurement Fig. S5b.

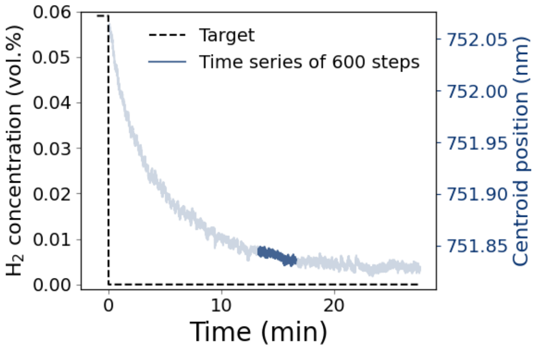


Figure S10: **Time series length for models optimized for accelerating sensor response.** Change in centroid position during the slowest occurring process in the training data, namely the desorption from 0.06 vol.% $H_2$ in measurement Fig. S4c. A time series comprising 600 time steps is chosen here to allow the model to estimate the rate of change in the spectrum, which is a prerequisite for accurately describing this process.

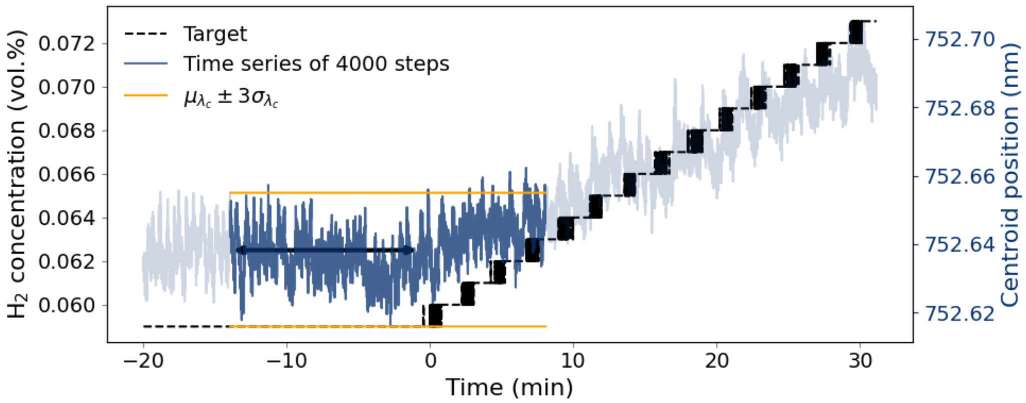


Figure S11: **Time series length for models optimized for leak detection.** The change in centroid position in the beginning of the leak with the smallest leak rate in Fig. S5a, compared to the mean and standard deviation of the centroid position before the leak has started (indicated by the double-headed arrow). Through using a time series comprising 4000 time steps the model should, in the worst case, be able to differentiate the leak occurring with the smallest slope from the noise in the sensor output data approximately 10 min after the leak has started.

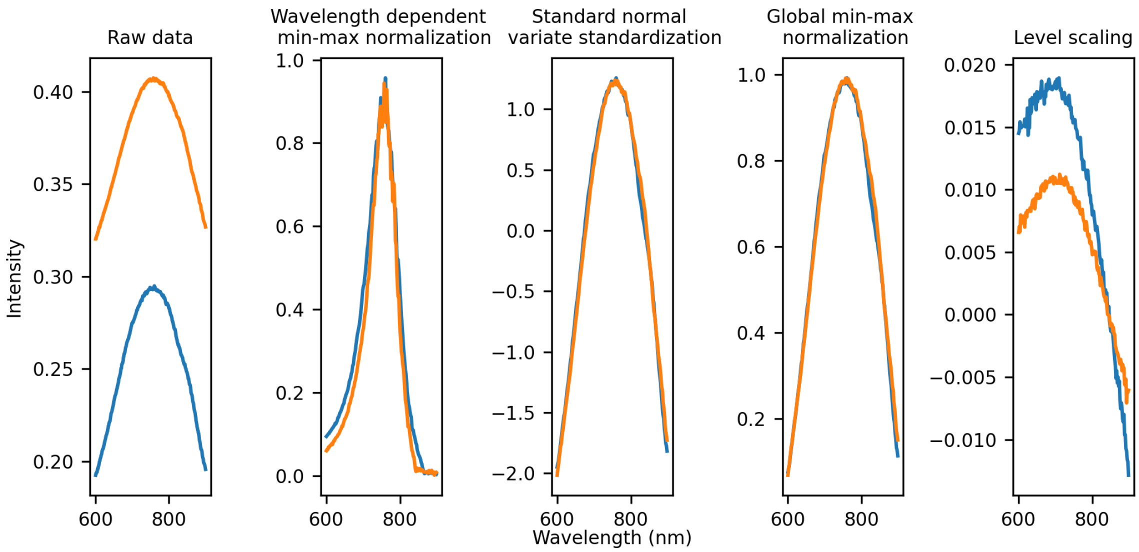


Figure S12: **Different pre-processing methods.** Illustration of the effect of different pre-processing methods on model prediction as well as raw data for spectra from measurement Fig. S4a (blue) and Fig. S4c (orange) at 0 vol.% $H_2$.

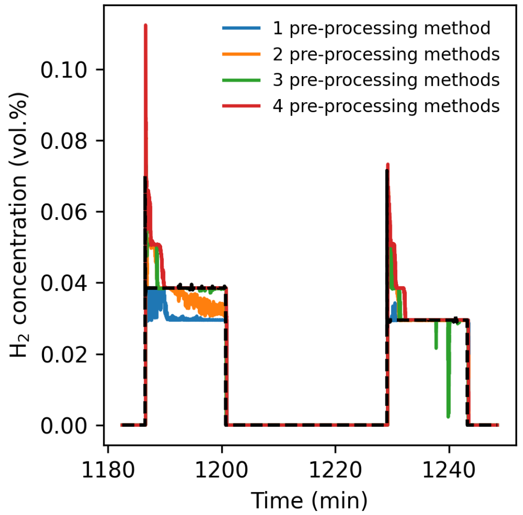


Figure S13: **Impact of using different pre-processing methods.** Predicted $H_2$ concentration on the two last step-wise increases in measurement Fig. S4c for models trained on the first half of measurement Fig. S4a and Fig. S4c, using different combinations of pre-processing methods.

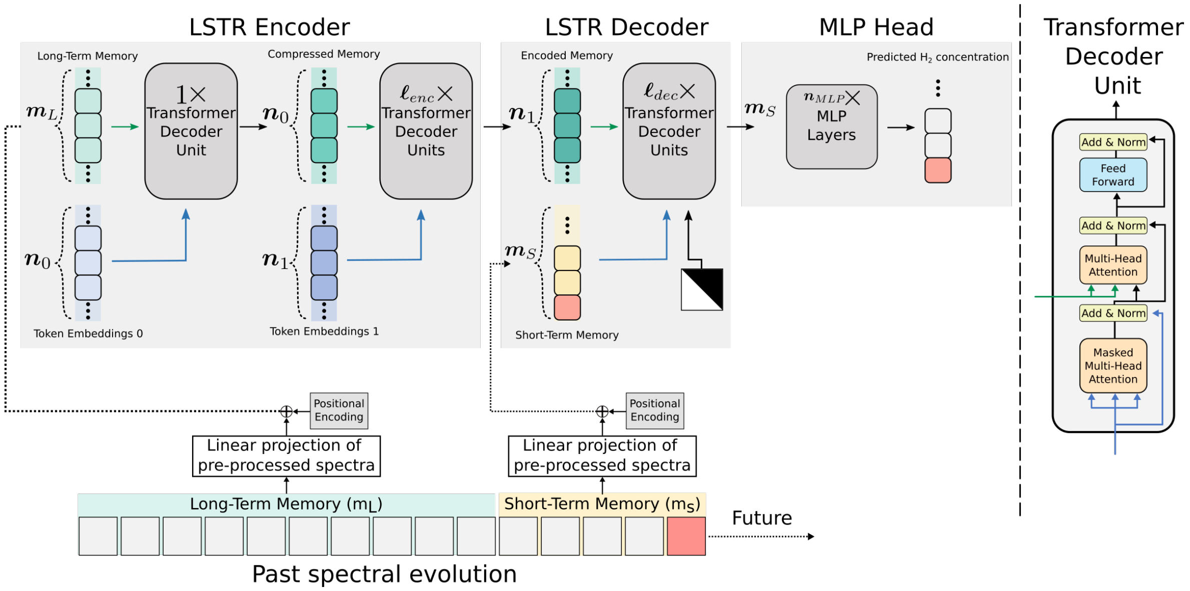


Figure S14: **Schematic illustration of the deep learning architecture used in this work.** Adapted from Ref. 2.

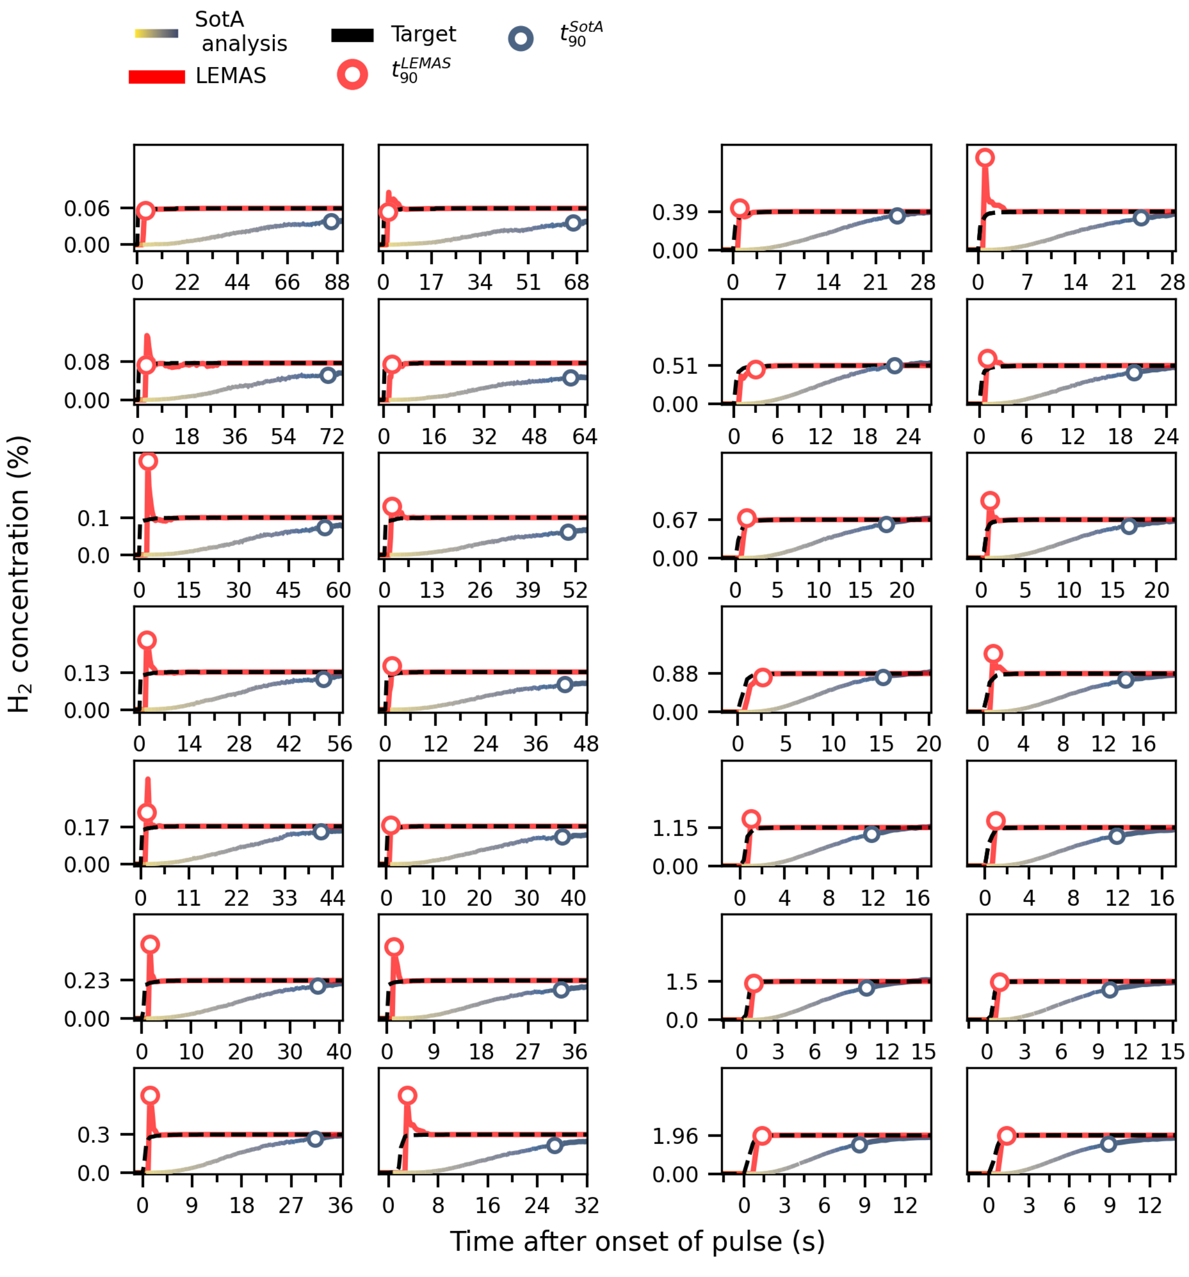


Figure S15: **Comparison of LEMAS and SotA analysis for step-wise increases in test data.**

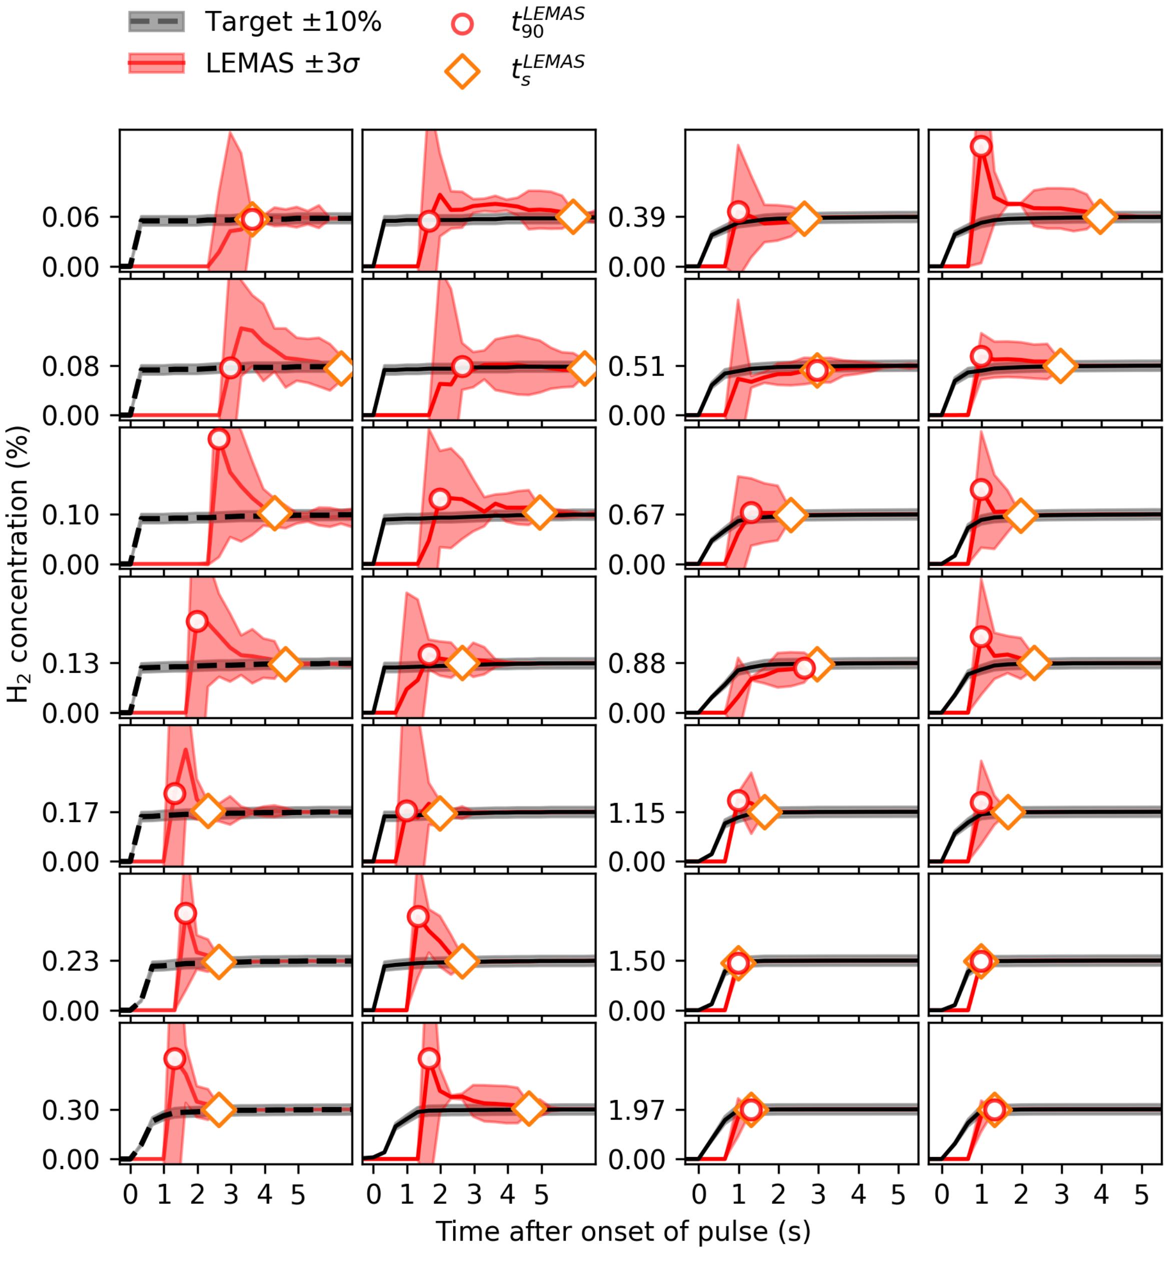


Figure S16: **Initial prediction of mean and standard deviation by LEMAS for step-wise increases in test data.**

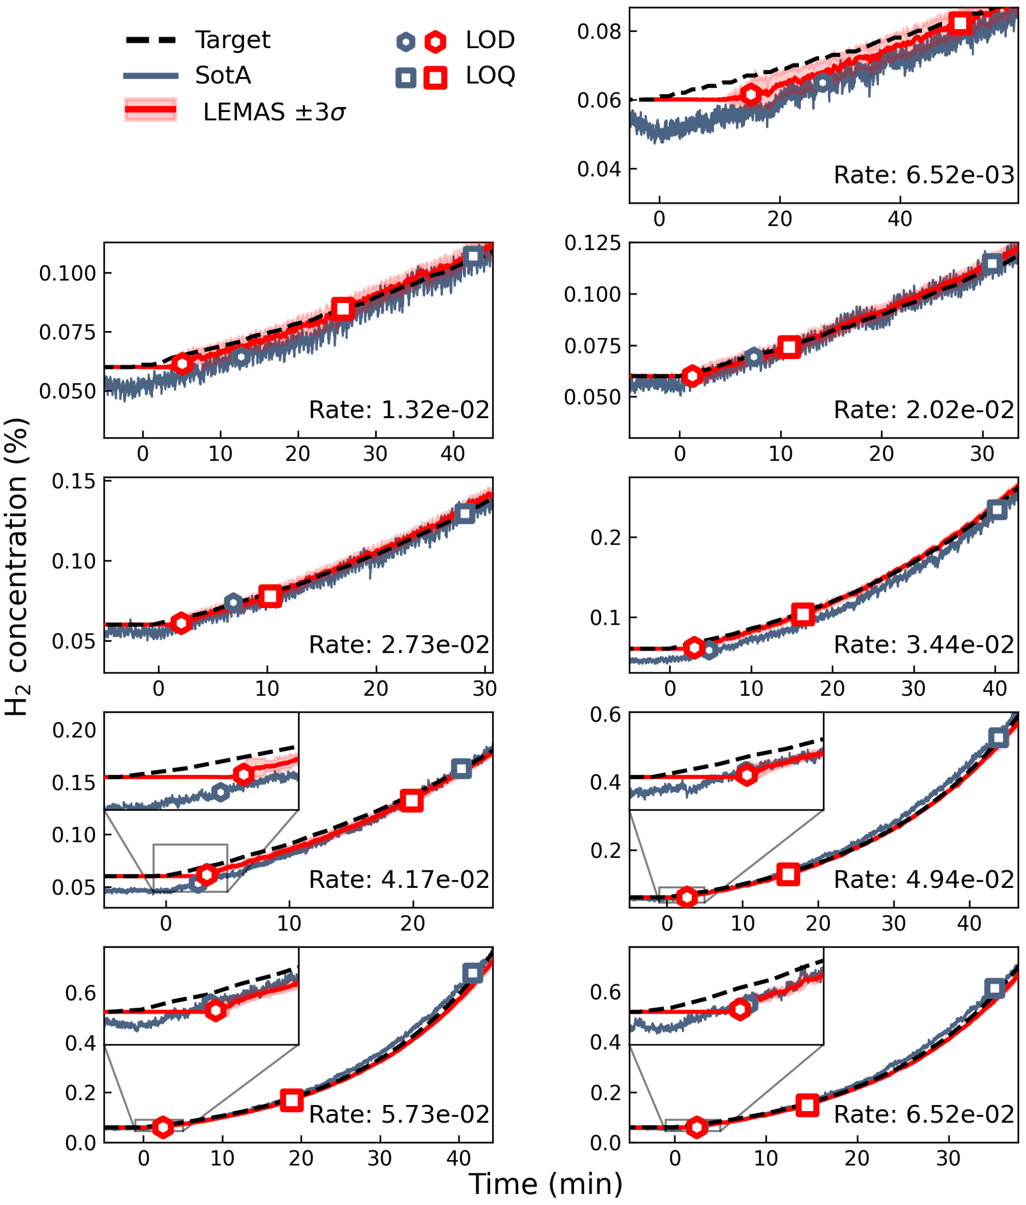


Figure S17: **Comparison of LEMAS and SotA analysis for exponential leak rates in test data.**

## Supplementary Tables

Table S1: **Hyperparameters used for all models.**

| Parameter | Value |
|---|---|
| $n_{\text{enc}}$ | 8 |
| $n_{\text{dec}}$ | 4 |
| $n_0$ | 8 |
| $n_1$ | 4 |
| $d_{\text{model}}$ | 256 |
| $d_{\text{ff}}$ | 512 |
| num heads | 8 |
| head size | 32 |
| Temporal stride on long term memory | 4 |
| $n_{\text{mlp}}$ | 8 |
| $d_{\text{mlp}}$ | 512 |
| Dropout rate | 0.1 |

## Supplementary References

[1] Iwan Darmadi. *Polymer-Nanoparticle Hybrid Materials for Plasmonic Hydrogen Detection.* PhD thesis, Chalmers University of Technology, Gothenburg, Sweden, January 2021. Available at `https://research.chalmers.se/en/publication/521833`.

[2] Mingze Xu, Yuanjun Xiong, Hao Chen, Xinyu Li, Wei Xia, Zhuowen Tu, and Stefano Soatto. Long short-term transformer for online action detection. In *NeurIPS 2021*, 2021. URL `https://www.amazon.science/publications/long-short-term-transformer-for-online-action-detection`.
